# Supplementary material for: FPT Approximations for Capacitated/Fair Clustering with Outliers
Source: arXiv:2305.01471 source file (2023-05-02)
Supplement: Supplementary file 1 [file fairappendix.tex]

%!TEX root = main.tex
\section{\texorpdfstring{Additional details for $(\fairone, \fairtwo)$-Fair $k$-Median with Outliers Problem}{Additional Details for Fair k-Median with Outliers}} \label{sec:fair-appendix}

\end{proof}
%\begin{theorem}
 %   There is an algorithm that computes an optimal fair assignment of a weighted set $\wtset$ of $n$ points to a set $\solution=\{f_1,f_2,\ldots,f_k\}$ facilities. That is, given a set $\solution \subseteq \facilities$ of size at most $k$ and the algorithm computes a assignment $\assign : \clients \times \solution \rightarrow \mathbb{Z}_{+}$ such that: The running time of algorithm is ...
%\end{theorem}
